# Supplementary material for: Building a Village: A Multi-stakeholder Approach to Open Innovation and Shared Governance to Promote Youth Online Safety
Source: arXiv:2504.03971 source file (2025-04-04)
Supplement: Supplementary file 1 [file 99-appendix-study3-alliances.tex]

\pagebreak\section{Youth Online Safety Organizations}\label{sec.alliances-study3}
The table below shows a non-exhaustive listing of organizations involved in youth online safety. The search terms used to find these organizations are ``\textit{youth online safety organizations commercial nonprofit government industry global}''.

%\begin{table}[htp]
\begin{longtable}{>{\raggedright}p{0.25\textwidth}>{\raggedright}p{0.40\textwidth}p{0.25\textwidth}}
%\small
%\begin{table}[H]
\caption{Youth Online Safety Organizations (Non-Exhaustive)}
\label{tab:alliances-study3}
%\centering
\small
%\begin{tabular}{llll}
%\begin{tabular}{>{\raggedright}p{0.15\textwidth}>{\raggedright}p{0.4\textwidth}p{0.2\textwidth}}
\\\toprule
%\hline
%\\\hhline{---}
\multicolumn{1}{l}{\textbf{Organization}} & \multicolumn{1}{l}{\textbf{Description}} & \multicolumn{1}{l}{\textbf{Link}}
%\textbf{Organization} & \textbf{Description}  & \textbf{Link} 
\\\midrule
\endfirsthead

\multicolumn{3}{c}%
{{\bfseries \tablename\ \ref{tab:alliances-study3} -- continued from previous page}} \\
\hline \multicolumn{1}{l}{\textbf{Organization}} & \multicolumn{1}{l}{\textbf{Description}} & \multicolumn{1}{l}{\textbf{Link}} \\ \midrule
\endhead

%\midrule
\multicolumn{3}{r}{{Continued on next page}}
\endfoot

\bottomrule
\endlastfoot

%org & desc & help & link \\\cline{1-3}\\
%org & desc & help & link \\\cline{1-3}
%org & desc & help & link 
Alannah \& Madeline Foundation & Australian charity promoting online safety through education, research, and community programs. & \url{https://www.amf.org.au/}\\\cline{1-3}
Australian Federal Police ThinkUKnow Program & Provides advice on youth social media safety and exploitation through a multi-agency collaboration. & \url{https://www.thinkuknow.org.au/}\\\cline{1-3}
Canadian Centre for Child Protection (C3P) & Provides education/resources to prevent social media child exploitation and online harassment. & \url{https://protectchildren.ca/}\\\cline{1-3}
Center for Cyber Safety and Education & Educates children on cybersecurity and online safety through Safe and Secure Online program. & \url{https://iamcybersafe.org/}\\\cline{1-3}
Childnet International & Advocates for safe social media use via resources for parents, educators, and youth. & \url{https://www.childnet.com/}\\\cline{1-3}
Children and Screens & Offers education and research on the impact of screen time on child development. & \url{https://www.childrenandscreens.com/}\\\cline{1-3}
Common Sense Media & Provides educational resources and advice to families for navigating digital media challenges. & \url{https://www.commonsensemedia.org/}\\\cline{1-3}
ConnectSafely & Offers guidance and safety tips for parents and teens on responsible social media use. & \url{https://www.connectsafely.org/}\\\cline{1-3}
Crimes Against Children Research Center (CCRC) & Conducts research on the prevalence and causes of crimes against children, including cybercrimes. & \url{https://www.unh.edu/ccrc/}\\\cline{1-3}
Cyber Civil Rights Initiative (CCRI) & Focuses on preventing/handling online harassment, especially image-based abuse. & \url{https://www.cybercivilrights.org/}\\\cline{1-3}
Cyberbullying Research Center & Conducts research on the causes and consequences of cyberbullying, providing resources to help prevent it. & \url{https://cyberbullying.org/}\\\cline{1-3}
eSafety Commissioner & Australia's regulator focused on reducing harmful social media behavior through education and regulation. & \url{https://www.esafety.gov.au/}\\\cline{1-3}
Family Online Safety Institute & Advocates for responsible use and promotes best practices to protect youth. & \url{https://www.fosi.org/}\\\cline{1-3}
Global Online Safety Regulators Network & An international coalition of regulators focusing on enhancing online safety across global platforms. & \url{https://www.globalsafetyregulators.org/}\\\cline{1-3}
Google Safety Center & Offers tools to help families and users manage privacy and safety across Google services. & \url{https://safety.google/}\\\cline{1-3}
Harvard Digital Thriving & Researches digital well-being among youth and provides educational resources for navigating online challenges. & \url{https://cyber.harvard.edu/}\\\cline{1-3}
INHOPE & Global network providing hotlines for reporting social media exploitation. & \url{https://www.inhope.org/}\\\cline{1-3}
Internet Matters & Offers advice and resources for families to keep children safe online. & \url{https://www.internetmatters.org/}\\\cline{1-3}
Internet Watch Foundation (IWF) & Identifies and removes child sexual abuse images and other harmful content. & \url{https://www.iwf.org.uk/}\\\cline{1-3}
MediaSmarts & Canadian organization providing digital literacy education for social media engagement. & \url{https://mediasmarts.ca/}\\\cline{1-3}
Meta Family Center & Provides parents and teens with resources for safe Facebook, Instagram, and Meta platform use. & \url{https://familycenter.meta.com/}\\\cline{1-3}
National Center for Missing \& Exploited Children (NCMEC) & Leads efforts to find missing children and prevent exploitation online. & \url{https://www.missingkids.org/}\\\cline{1-3}
National Cyber Security Alliance & Promotes cybersecurity education via partnerships with tech companies and governments. & \url{https://staysafeonline.org/}\\\cline{1-3}
National Network to End Domestic Violence (NNEDV) & Offers guides and advocacy for protecting youth from tech-related abuse. & \url{https://www.nnedv.org/}\\\cline{1-3}
National Parent Teacher Association (PTA) & Advocates for social media safety among families through education and policy efforts. & \url{https://www.pta.org/}\\\cline{1-3}
NetSmartz & Provides age-appropriate resources for teaching children how to be safer online. & \url{https://www.missingkids.org/netsmartz}\\\cline{1-3}
Organization for Social Media Safety & Advocates for safety measures across social media platforms to protect users, especially children. & \url{https://www.ofsms.org/}\\\cline{1-3}
Parent Zone & Provides educative material based on academic and independent research & \url{https://parentzone.org.uk/}\\\cline{1-3}
Safer Internet Centre & Operates a UK-wide helpline and resources for social media safety. & \url{https://www.saferinternet.org.uk/}\\\cline{1-3}
Save the Children (Norway) & Offers education to prevent social media exploitation, particularly in humanitarian contexts. & \url{https://www.reddbarna.no/}\\\cline{1-3}
StopBullying.gov & Provides info to prevent and respond to bullying, including cyberbullying. & \url{https://www.stopbullying.gov/}\\\cline{1-3}
Technology Coalition & Unites tech companies to develop strategies/resources to combat child exploitation. & \url{https://www.technologycoalition.org/}\\\cline{1-3}
Thorn & Develops tech and programs to combat online child sexual abuse and exploitation. & \url{https://www.thorn.org/}\\\cline{1-3}
UNICEF & Technology stream to end cyberbullying. & \url{https://www.unicef.org/innovation/kindly} \\

       %\\  \bottomrule
%\end{tabular}

\end{longtable}
