# Supplementary material for: Building a Village: A Multi-stakeholder Approach to Open Innovation and Shared Governance to Promote Youth Online Safety
Source: arXiv:2504.03971 source file (2025-04-04)
Supplement: Supplementary file 2 [file 99-appendix-study3-glossary.tex]

\pagebreak
\section{Acronyms and Glossary}\label{sec.study3-glossary}
\printglossary[type=\acronymtype]

%\printglossary[type=\acronymtype,title=\listofacronyms, toctitle=\listacronyms]
%\addacronymx

%\printglossary[title=\listofglossary]
\printglossary
%\clearpage\begingroup\let\newpage\relax\printglossary[title=\listglossary, toctitle=\listglossary]\endgroup
%\printglossary[title=\listofglossary, toctitle=\listglossary]
%\addglossaryx
